# Supplementary material for: Laser Cooling of Molecular Anions
Source: arXiv:1506.06505 source file (2015-06-22)
Supplement: Supplementary file 1 [file Supplementary.pdf]

# Laser Cooling of Molecular Anions

Pauline Yzombard[1], Mehdi Hamamda[1], Sebastian Gerber[2], Michael Doser[2] and Daniel Comparat[1]
(Dated: May 28, 2015)

## I. SUPPLEMENTARY MATERIAL

Table I reviews most of the experimental as well as theoretical studies of diatomic anions with useful references if further studies are needed.

We found that the states of light anions with s or p electrons are often similar to the states of their isoelectronic neutral species [1].

However, anions containing metal atoms with d electrons are more complex and often exhibit several stable states [2]. The electronic structure given in the table is only a "typical" one [3]; exceptions exist and are sometimes given in the list. Heavy molecules usually possess more bound states than light ones but sometimes with a different ground state.

| O.E. | Neutral | Electronic Structure | group | example |
|---|---|---|---|---|
| 3 | BeH | $X^2\Sigma$ ($A^2\Pi$) ($B^2\Pi$) | I-I | $H_2^-$ (unstable)[4] $Li_2^-$[5] $LiH^-$ $NaH^-$[6] LiNa−[7] $Cu_2^-$ $Ag_2^-$[8] $Au_2^-$[9] |
| 4 | BH | $X^1\Sigma$ (a $^3\Pi$) ($A^1\Pi$) | I-II | $BeH^-$ $MgH^-$ [10–12] $CaH^-$[11] $LiBe^-$ $LiMg^-$[7] $BeNa^-$ $MgNa^-$ [13] |
| 5 | CH | $^2\Pi$ $^4\Sigma$ | I-III | $BH^-$[14] $AlH^-$ $AlLi^-$[1] $AlNa^-$ $AlK^-$ [15] $LiB^-$[7] |
| | | $^2\Pi$ | II-II | $Be_2^-$[16] |
| 6 | NH | $X^3\Sigma^-$ $a^1\Delta$ $b^1\Sigma^+$ ($A^3\Pi$) | I-IV | $LiC^-$ $LiSi^-$[7] $CH^-$ $SiH^-$ $GeH^-$[17, 18] $CNa^-$ $SiNa^-$($^3\Sigma^5\Sigma$ dipole bound)[19, 20] |
| | | | | $SiCu^-$ $SiAg^-$, $SiAu^-$ [20] |
| | | | II-III | $AlBe^-$ [1] $AlMg^-$ $AlCa^-$ $AlSr^-$ $AlBa^-$ [15] |
| 7 | OH | $X^2\Pi$ $A^2\Sigma$ $B^2\Sigma$ or $X^4\Sigma$ | I-V | $LiN^-$[7] $PH^-$[21, 22] |
| | | | II-IV | $BeC^-$ $MgSi^-$[23] $SiBe^-$ $CMg^-$ $SiMg^-$ [20] |
| | | $X^4\Sigma$ $a^2\Pi$ $^2\Sigma$ $^2\Delta$ | III-III | $B_2^-$[24, 25] $Al_2^-$ $Ga_2^-$[26] $AlB^-$[1] |
| 8 | $C_2$ | $X^1\Sigma$ or $^3\Pi$ ($^1\Pi$ $^3\Sigma$) | I-VI | $OH^-$ $SH^-$ $SeH^-$ $TeH^-$[27] $LiO^-$[28, 29] $LiS^-$[7] $NaO^-$ $KO^-$($X^1\Sigma^+$)[29, 30] |
| | | | | $CuO^-$ $AgO^-$ $AuS^-$[31] $CrH^-$[2] $AuO^-$ $AuS^-$[32] |
| | | $^3\Pi$ $^3\Sigma$ $^1\Sigma$ | III-IV | $BC^-$[14] $AlC^-$[1] |
| 9 | CN | $X^2\Sigma^+$ $A^2\Pi$ $B^2\Sigma^+$ | I-VII | $LiF^-$ $LiCl^-$ $NaF^-$ $NaCl^-$[6, 6, 7] $MnH^-$($X^6\Delta$)[33] |
| | SrF | | II-VI | $ZnO^-$[20, 34] $BeO^-$ $MgO^-$[35] $ZnF^-$[34, 36] |
| | | + $^4$ states | III-V | $BP^-$[37] $AlN^-$ $AlP^-$ $AlAs^-$ [38–40] $GaP^-$ $InP^-$ $GaAs^-$ [41] $BN^-$[42] $GaN^-$[43] |
| | | | IV-IV | $C_2^-$[44] $Si_2^-$[45] $CSi^-$(B unstable)[46, 47] $Sn_2^-$ $Pb_2^-$ $SnPb^-$($X^2\Pi$) [48] |
| 10 | $N_2$ | $^1\Sigma$ $^3\Pi$ ($^3\Sigma$) ($^3\Delta$) | I-VIII | $HeH^-$$NeH^-$$ArH^-$[11] $FeH^-$ $NiH^-$[2, 33] $CoH^-$($X^4\Phi$)[49] $NiCu^-$($X^3\Delta$) $AgNi^-$[50] |
| | CO | | II-VII | $BeF^-$ (unstable)[51] $MgCl^-$[52] |
| | | | III-VI | $BO^-$[53, 54] $AlO^-$[1] $ScO^-$ [20] |
| | | | IV-V | $CN^-$[54, 55] $SiN^-$[56] $CP^-$ $CAs^-$ $SiP^-$ $SiAs^-$ $GeP^-$ $GeAs^-$[23] |
| 11 | NO | $^2\Pi$ $^4\Pi$ $^2\Sigma$ | III-VII | $BF^-$(unstable)[57] $AlF^-$[1] |
| | CF | | IV-VI | $CO^-$(unstable)[57] $CS^-$[58] $SiO^-$[59] $SnO^-$[60] $CS^-$ $CSe^-$ $GeO^-$ $GeS^-$ $GeSe^-$[23] $TiO^-$[20] |
| | | | V-V | $N_2^-$ (unstable)[57] $PN^-$[59] |
| 12 | NF | $X^3\Sigma^-$ $a^1\Delta$ $b^1\Sigma^+$ | IV-VII | $SiF^-$ $CCl^-$[61] |
| | $O_2$ | | V-VI | $NO^-$[62] $PO^-$ $NS^-$ $PS^-$[63, 64] $NSe^-$ $PS^-$ $PSe^-$ $AsO^-$ $AsS^-$ $AsSe^-$[23] $VO^-$ [20] |
| 13 | OF | $X^2\Pi$ | V-VII | $NF^-$[65] $PF^-$ $PCl^-$[22] |
| | SF | | VI-VI | $O_2^-$[54, 66] $Se_2^-$ $SeS^-$[67] $S_2^-$[65] $SO^-$[68] $CrO^-$ [20] |
| 14 | $F_2$ | $X^1\Sigma^+$ $a^3\Pi$ $A^1\Pi$ | V-VIII | $PtN^-$[69] |
| | $Cl_2$ | | VI-VII | $OF^-$ $SF^-$[65] $BrO^-$ $IO^-$[70] $ClO^-$[71, 72] $MnO^-$ [20] |
| 15 | NeF | all types of X states | VI-VIII | $HeO^-$ $ArO^-$ $NeO^-$[73] $KrO^-$[74] $FeO^-$[75] $NiO^-$[76] $PdO^-$[77] $CoO^-$[78] $PtO^-$[79] |
| | XeCl | $X^2\Sigma$ $A^2\Pi$ $B^2\Sigma$ | VII-VII | $F_2^-$[65, 80] $I_2^-$[81, 82] $IBr^-$[83, 84] $BrF^-$ $BrCl^-$ $ClF^-$[85] $Cl_2^-$[86] |
| 16 | $Ne_2$ | Van der Walls X1/2 | VII-VIII | $IXe^-$[87] $KrBr^-$ $XeBr^-$ $KrCl^-$ $KrI^-$ $ArI^-$ $IHe^-$ $INe^-$ $BrHe^-$ $BrNe^-$ $BrAr^-$[88] |
| | | | | $FHe^-$ $FNe^-$ $FAr^-$[89] $ArBr^-$[90] $IXe^-$[91] $HeCl^-$ $NeCl^-$ $ArCl^-$ $KrCl^-$[92] |
| 17 | | multiple states | VIII-VIII | $He_2^-$(unstable)[93] $Ni_2^-$ $Pd_2^-$ $Pt_2^-$[94] $Fe_2^-$ $Co_2^-$[95] |

TABLE I: Some properties of some diatomic anionic molecules. O.E. designates the number of outermost electrons for the anionic system $AB^-$. A typical, well known, neutral molecule with the same number of O.E. is then given. Groups of atoms (using the Chemical Abstracts Service (CAS) notation) are: I (H, Li, Na,..., Cu, Ag,...), II(Be, Mg,..., Zn, Cd,...) III(B,Al,Ga,..., Sc, Y, ...), IV (C,Si,Ge,Sn, ..., Ti, Zr,...), V(N,P,As,..., V, Nb,...), VI (O,S,Se,..., Cr, Mo,...), VII (F, Cl, Br,..., Mn Tc,...), VIII(He, Ne, Ar,... Fe, Co, Ni,...). We recall that molecules formed with C, O, Mg, Si, S, Ca, Ti, Cr, Fe ... atoms have no hyperfine structure (for the most abundant isotopes). The typical electronic structure is given; usually unstable states are indicated in parentheses. Some examples of anions having a given number of O.E. are given.

Fortunately, for laser cooling purposes, several diatomic molecules AB possess more than one stable electronic anionic $AB^-$ bound state, often due to a large electron affinity [96] and to a competition between energetically close configurations or multiplets [63]. However, the spectroscopic studies are usually partial and often only theoretical or consider only the ground state.

As discussed in the main text several systems with 8, 14 or higher number of outermost electrons or with e.g. O, Li or Al atoms [1, 7] look theoretically interesting, with Franck-Condon factors of more than 70% but have transitions that probably lie in the infrared region. There is thus clearly a need for new experimental, as well as theoretical, data in order to choose the best candidate for laser cooling.

---


[1] G. L. Gutsev *et al.*, J. Chem. Phys. **110**, 2928 (1999).
[2] A. E. S. Miller *et al.*, J. Chem. Phys. **87**, 1549 (1987).
[3] A. I. Boldyrev *et al.*, J. Phys. Chem. **98**, 9931 (1994).
[4] O. Heber *et al.*, Phys. Rev. A **73**, 60501 (2006).
[5] H. H. Michels *et al.*, Chem. Phys. Lett. **118**, 67 (1985).
[6] G. L. Gutsev *et al.*, Chem. Phys. Lett. **276**, 13 (1997).
[7] A. I. Boldyrev *et al.*, J. Chem. Phys. **99**, 8793 (1993).
[8] J. Ho *et al.*, J. Chem. Phys. **93**, 6987 (1990).
[9] I. León *et al.*, J. Chem. Phys. **139**, 194306 (2013).
[10] R. Rackwitz *et al.*, Z. Naturforsch. A **32**, 594 (1977).
[11] J. P. Harris *et al.*, J. Chem. Phys. **140**, 84304 (2014).
[12] A. Buytendyk *et al.*, International Journal of Mass Spectrometry **365**, 140 (2014).
[13] C. W. Bauschlicher *et al.*, J. Chem. Phys. **96**, 1240 (1992).
[14] C. J. Reid, International Journal of Mass Spectrometry **127**, 147 (1993).
[15] J. Wang *et al.*, Theoretical Chemistry Accounts **121**, 165 (2008).
[16] I. G. Kaplan *et al.*, J. Chem. Phys. **117**, 3687 (2002).
[17] C. J. Reid, J. Phys. B **26**, 2359 (1993).
[18] P. J. Bruna *et al.*, J. Mol. Struct. **599**, 261 (2001).
[19] J. Kalcher *et al.*, Can. J. Chem **326**, 80 (2000).
[20] J. Kalcher Annu. Rep. Prog. Chem., Sect. C: Phys. Chem. **97**, 149 (2001).
[21] P. F. Zittel *et al.*, J. Chem. Phys. **65**, 1236 (1976).
[22] M. T. Nguyen, Mol. Phys. **59**, 547 (1986).
[23] J. Kalcher, Phys. Chem. Chem. Phys. **4**, 3311-3317 (2002).
[24] P. J. Bruna *et al.*, J. Phys. B **23**, 2197 (1990).
[25] E. Miliordos *et al.*, J. Chem. Phys. **132**, (2010).
[26] A. C. Stowe *et al.*, J. Chem. Phys. **115**, 4632 (2001).
[27] C. Mungan, J. Phys. Chem. Solids **56**, 735 (1995).
[28] Z. Tian *et al.*, Proceedings of the National Academy of Sciences **105**, 7647 (2008).
[29] B. Mintz *et al.*, J. Phys. Chem. A **113**, 9501 (2009).
[30] C. W. Bauschlicher Jr *et al.*, J. Chem. Phys. **99**, 3654 (1993).
[31] D. H. Andrews, *Anion Photoelectron Spectroscopy*, PhD thesis, University of Colorado, 2006.
[32] T. Ichino *et al.*, J. Phys. Chem. A **108**, 11307 (2004).
[33] A. E. Stevens *et al.*, J. Chem. Phys. **78**, 5420 (1983).
[34] V. D. Moravec *et al.*, Chem. Phys. Lett. **341**, 313 (2001).
[35] J. H. Kim *et al.*, J. Phys. Chem. A **105**, 5709 (2001).
[36] S. Hayashi, *et al.*, J. Chem. Phys. **129**, 44313 (2008).
[37] R. Linguerri *et al.*, Chem. Phys. **346**, 1 (2008).
[38] P. J. Bruna *et al.*, J. Phys. B **22**, 1913 (1989).
[39] P. J. Bruna *et al.*, J. Phys. Chem. A **105**, 3328 (2001).
[40] C. M. Clouthier *et al.*, J. Mol. Spectrosc. **219**, 58 (2003).
[41] H. Gomez *et al.*, J. Chem. Phys. **117**, 8644 (2002).
[42] R. C. Mawhinney *et al.*, Can. J. Chem. **71**, 1581 (1993).
[43] P. A. Denis *et al.*, Chem. Phys. Lett. **423**, 247 (2006).
[44] M. Tulej *et al.*, Journal of Raman Spectroscopy **41**, 853 (2010).
[45] H. Liu *et al.*, Spectrochim. Acta Part A **108**, 295 (2013).
[46] A. Pramanik *et al.*, Chem. Phys. Lett. **468**, 124 (2009).
[47] R. C. Bilodeau *et al.*, Chem. Phys. Lett. **426**, 237 (2006).
[48] J. Ho *et al.*, J. Chem. Phys. **96**, 144 (1992).
[49] C. N. Sakellaris *et al.*, J. Chem. Phys. **137**, 34309 (2012).
[50] S. J. Dixon-Warren *et al.*, J. Chem. Phys. **104**, 4902 (1996).
[51] X.-L. Zhao *et al.*, Nucl. Instrum. Methods. Phys. B **259**, 345 (2007).
[52] T. M. Miller *et al.*, Chem. Phys. Lett. **146**, 364 (1988).
[53] L. H. Andersen *et al.*, J. Chem. Phys. **115**, 3566 (2001).
[54] H. Deutsch *et al.*, International Journal of Mass Spectrometry **277**, 151 (2008).
[55] J. Tellinghuisen *et al.*, J. Chem. Phys. **91**, 5476 (1989).
[56] G. Meloni *et al.*, J. Phys. Chem. A **108**, 9750 (2004).
[57] A. Dreuw *et al.*, J. Chem. Phys. **116**, 6039 (2002).
[58] M. Hochlaf *et al.*, J. Chem. Phys. **110**, 11835 (1999).
[59] G. L. Gutsev *et al.*, Phys. Rev. A**58**, 4972 (1998).
[60] G. E. Davico *et al.*, J. Chem. Phys. **113**, 8852 (2000).
[61] K. A. Peterson *et al.*, J. Chem. Phys. **93**, 1876 (1990).
[62] R. Polák *et al.*, Chemical Physics **303**, 73 (2004).
[63] P. J. Bruna *et al.*, J. Phys. B **20**, 5967 (1987).
[64] S. Ben Yaghlane *et al.*, J. Phys. B **38**, 3395 (2005).
[65] J. Czernek *et al.*, Chem. Phys. **303**, 137 (2004).
[66] J. A. Sordo, J. Chem. Phys. **114**, 1974 (2001).
[67] M. Ikezawa *et al.*, J. Chem. Phys. **58**, 2024 (1973).
[68] M. L. Polak *et al.*, J. Chem. Phys. **94**, 6926 (1991).
[69] K. K. Murray *et al.*, Phys. Rev. A **36**, 699 (1987).
[70] M. K. Gilles *et al.*, J. Chem. Phys. **96**, 8012 (1992).
[71] S.-J. Kim *et al.*, J. Chem. Phys. **117**, 9703 (2002).
[72] Z. Noorisafa *et al.*, Spectrochim. Acta Part A (2014).
[73] L. A. Viehland *et al.*, J Chem Phys. **122**, 114302 (2005).
[74] E. Garand *et al.*, J.Phys. Chem. A **113**, 14439 (2009).
[75] C. N. Sakellaris *et al.*, J. Chem. Phys. **134**, 234308 (2011).
[76] C. N. Sakellaris *et al.*, J. Chem. Phys. **138**, 54308 (2013).
[77] S. A. Klopcic *et al.*, J. Chem. Phys. **110**, 10216 (1999).
[78] C. N. Sakellaris *et al.*, J. Phys. Chem. A **116**, 6935 (2012).
[79] T. M. Ramond *et al.*, J. Mol. Spectrosc. **216**, 1 (2002).
[80] N. S. Shuman *et al.*, Phys. Rev. A**88**, 62708 (2013).
[81] M. T. Zanni *et al.*, J. Chem. Phys. **107**, 7613 (1997).
[82] S. B. Sharp *et al.*, Mol. Phys. **98**, 667 (2000).
[83] J. Simons, J. Phys. Chem. A **112**, 6401 (2008).
[84] J. Simons, Ann. Rev. Phys. Chem. **62**, 107 (2011).
[85] T. J. Van Huis *et al.*, Mol. Phys. **89**, 607 (1996).
[86] H. Sabzyan *et al.*, Spectrochim. Acta Part A **117**, 95 (2014).

[87] T. Lenzer *et al.*, J. Chem. Phys. **109**, 10754 (1998).
[88] A. A. Buchachenko *et al.*, J. Chem. Phys. **122**, 194311 (2005).
[89] B. R. Gray *et al.*, Phys. Chem. Chem. Phys. **8**, 4752 (2006).
[90] A. A. Buchachenko *et al.*, J. Chem. Phys. **128**, (2008).
[91] G. J. Hoffman, Chem. Phys. **361**, 68 (2009).
[92] N. C. Bera *et al.*, Mol. Phys. **105**, 1433 (2007).
[93] T. Andersen *et al.*, J. Phys. B **27**, 1135 (1994).
[94] J. Ho *et al.*, J. Chem. Phys. **99**, 8542 (1993).
[95] D. G. Leopold *et al.*, J. Chem. Phys. **85**, 51 (1986).
[96] J. C. Rienstra-Kiracofe *et al.*, Chem. Rev. **102**, 231 (2002).
